# Supplementary material for: DiscoSense: Commonsense Reasoning with Discourse Connectives
Source: arXiv:2210.12478 source file (2022-10-22)
Supplement: Supplementary file 1 [file data.tex]

\comment{
\section{Discourse Markers in \textsc{Discosense}}
In this section, we present a list of markers that are present within \textsc{Discosense}. Amongst 174 discourse markers present within \textsc{Discovery}, we filter out discourse markers that can give rise to multiple plausible endings or sentences with multiple interpretations. We retain a total of 37 discourse markers as listed out in ~\autoref{tab:markers_list}.

\begin{table}[t!]
\begin{center}
\begin{tabular}{lll}
\toprule
Markers \\ \midrule
as a result \\
by contrast \\
because of this \\
because of that \\
but \\
however \\
in contrast \\
consequently \\
for example \\
for instance \\
hence \\
likewise \\
rather \\
conversely \\
interestingly \\
though \\
yet \\
although \\
nonetheless \\
thereby \\
on the contrary \\
in sum \\
subsequently \\
particularly \\
in other words \\
in particular        \\
instead \\
inshort \\
nevertheless \\
overall \\
otherwise \\
on the other hand \\
similarly \\
specifically \\
therefore         \\
thereafter \\
thus \\
\bottomrule
\end{tabular}
\end{center}
\caption{Discourse markers present within \textsc{DiscoSense}.}
\label{tab:markers_list}
\end{table}
}

\comment{
\section{Distribution of Discourse Markers}

We report the distribution of discourse marker across the training and test sets in ~\autoref{fig:training_marker_stats} of \textsc{DiscoSense}. The most and least frequently present discourse markers in training set are 'instead' and 'thereby' with frequency of 570 and 106 respectively.

\begin{figure}[!t]
\centering
    \includegraphics[height=0.8\linewidth, scale=0.14]{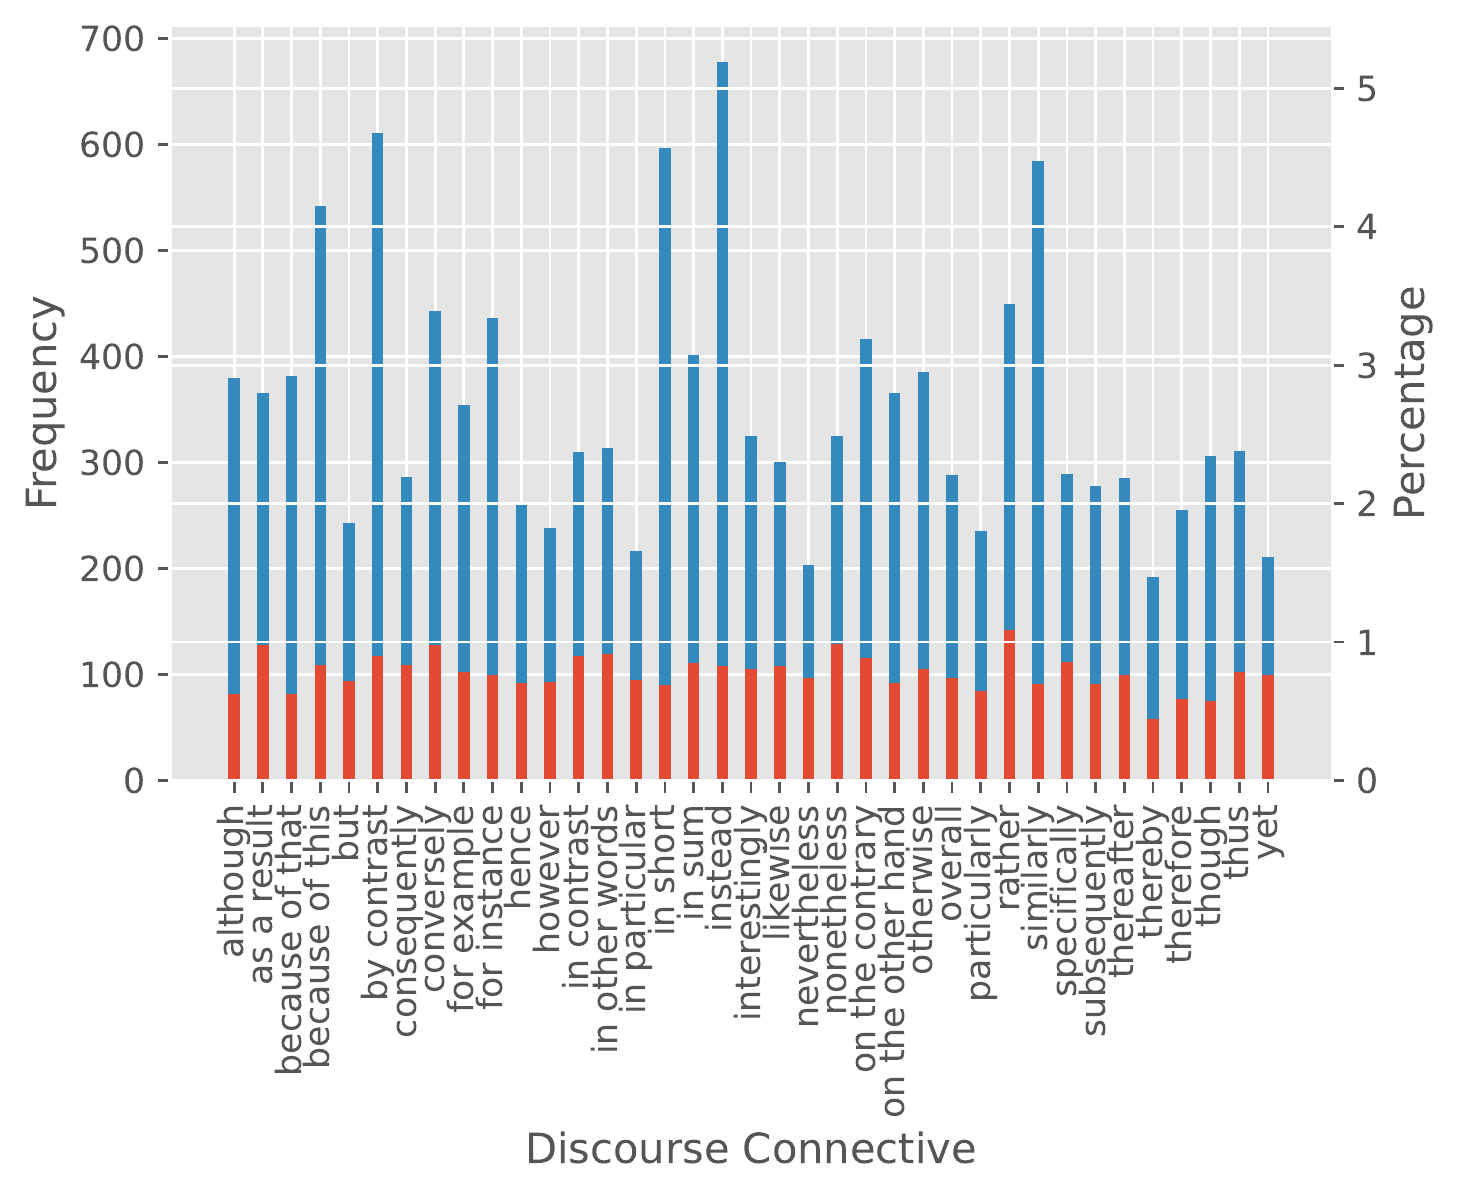}
  \caption{Distribution of discourse marker across \textsc{DiscoSense}.}
\label{fig:training_marker_stats}
\end{figure}

\section{How is \textsc{DiscoSense} different from existing commonsense reasoning benchmarks?}
In this section, we mention salient features of \textsc{DiscoSense} which makes it different from existing commonsense reasoning datasets.

\comment{
\textbf{Contextual sentences: }
Many context sentences in DiscoSense do not start afresh and have a higher degree of context attached with them. Compared to SocialIQA in which examples are constructed from well defined event phrases from ATOMIC Knowledge Base \cite{Hwang2021COMETATOMIC2O} or Abductive NLI wherein instances are constructed from stories from RocStories \cite{mostafazadeh-etal-2016-corpus} that have a clear beginning, DiscoSense contains examples that do not necessarily provide all the background within the context to answer the question. \autoref{fig:contextual_example} gives an example (more examples can be found in ~\autoref{tab:abductive_examples}), wherein the context straight away talks about finalization of some standards and asks why competitor was able to finish their task on time. Sentences of this type only provide the required context necessary to arrive at the correct label and prompts LM to related prior world knowledge with abductive/linguistic commonsense reasoning.
}

\paragraph{Improved quality of generated sentences.} Compared to existing commonsense reasoning datasets, \textsc{DiscoSense} features higher quality text sentences due to drastically better generator (\textsc{Gpt} vs \textsc{Ctrl}) and discriminator LMs (\textsc{Bert-large} vs \textsc{Roberta large}) used in creating it. The discriminator \textsc{Roberta} \cite{liu2019roberta} used in our work has been shown to significantly outperform \textsc{Bert} on all tested downstream tasks. Our generator contains nearly 15x more parameters trained on 28x more data than the previously best used generator \textsc{Gpt} for creating synthetic distractors. Moreover the conditional training approach outperforms unconditionally trained approach drastically in terms of perplexity (see line 335 in Section~3.3.1).
%\autoref{tab:perplexity}. 
This claim aligns with algorithmic perspective mentioned in \citet{zellers-etal-2019-hellaswag} wherein it was discussed that using better discriminator/generator LMs are bound to create a more robust adversarial dataset than the one created using less powerful LMs.

\paragraph{Wider components of commonsense reasoning.} Unlike existing Commonsense reasoning datasets that target a specific component of reasoning explicitly such as \textsc{SocialIQA}/ \textsc{Abductive NLI}/\textsc{Piqa} or focus on temporal reasoning (\textsc{Swag}/\textsc{Hellaswag}), \textsc{DiscoSense} features examples that aim to evaluate numerous components of commonsense reasoning. We provide examples from the training set of \textsc{DiscoSense} belonging to numerous categories:

\begin{itemize}
\item Physical World Reasoning:  This type of reasoning aims to evaluate neural models on their knowledge of physical commonsense. 
%We showcase these examples in ~\autoref{tab:physical_world_examples}. 
These examples are concerned more with everyday situations and are concerned with physical aspects of our world.
\item Social Commonsense Reasoning: This category of examples 
%(shown in ~\autoref{tab:social_examples})  
examines how well neural models can perform commonsense reasoning about social situations. 
\item Numerical Reasoning: This category of examples examines how well neural models can learn to perform numerical reasoning. Examples %(shown in ~\autoref{tab:numerical_examples})
require identifying numerical aspect from a context and figuring out how it is connected to the overall context.
\item Linguistic Reasoning: This type of examples %(shown in ~\autoref{tab:linguistic_examples})
are focused on evaluating how well neural models can perform reasoning over intricate texts.
\item Temporal Reasoning: This category of examples examines temporal commonsense comprehension of neural models. In these examples, %(shown in ~\autoref{tab:temporal_examples}), 
it is crucial to figure out what impact time has had on the subjects of context and understanding what role it plays within the context to determine the answer.
\item Abductive Reasoning: This category of examples aims to assessing how well can neural LMs can come up with most plausible observation in the presence of incomplete observations. 
%We show examples belonging to this category in ~\autoref{tab:abductive_examples}.\\
This allows this benchmark to be used for evaluating how LMs capture all these broader components of commonsense reasoning.
% such as social ~\autoref{fig:social_example_main} (more in ~\autoref{tab:social_examples}), physical world (~\autoref{tab:physical_world_examples}), linguistic (~\autoref{tab:linguistic_examples}), numerical (~\autoref{tab:numerical_examples}), temporal (~\autoref{tab:temporal_examples}) and abductive (~\autoref{tab:abductive_examples} reasoning. 
\end{itemize}

\paragraph{Increased Inference Step/Complexity:}
It has been widely studied that the performance of PLMs on downstream tasks deteriorate when the number of inference step increases \cite{richardson-sabharwal-2020-qa, DBLP:conf/aaai/ZhouZCH20, huang-etal-2019-cosmos}. Each example in \textsc{DiscoSense} requires a PLM to understand the role of a discourse marker to arrive at the correct label. Compared to the standard task of attending to context like in \textsc{Swag} and \textsc{Hellaswag}, the additional task of performing reasoning over a discourse marker contributes to an additional inference step making the task harder. Removing biases and adding extra inference step make it hard for PLMs to be right for wrong reasons \cite{mccoy-etal-2019-right}.
}

\comment{
\section{Crowdsourcing Details}
We perform crowdsourcing to validate if humans are able to identify the ground truth in each example present in training and test sets of \textsc{DiscoSense}. Since in each example three options have been synthetically generated, it is crucial to ensure that humans are able to identify which ending is human generated (ground truth) and which ones have been generated by generator LMs. Since the primary task in \textsc{DiscoSense} is to determine the most plausible ending given a context and a discourse marker, we formally define what we mean by 'most plausible ending'. Specifically:

%Our definition of most plausible ending is similar to the one used in \textsc{HellaSwag} \cite{zellers-etal-2019-hellaswag}. Annotators are required to choose ending which they perceive as most feasible amongst all 4 endings. Using the annotator's definition of commonsense, they are asked to assign confidence scores to all 4 endings. If two or more endings seem equally feasible, they were asked to use the following criteria:

\begin{enumerate}
    \item The most plausible ending needs to be the strongest statement (least number of counterarguments). If an ending is fallible, that should not be marked as the correct option. In this case, workers prefer the statement which has the least/or no direct flaws. This complies with the definition of commonsense knowledge that it needs to be agreed on by many people.
    \item The most plausible ending cannot be inconsistent with the context and needs to comply with the purpose of the discourse marker.
    %\item Each human verifier has to read all four options along with assignment of confidence scores on each option. Filter out the endings that are either less plausible or have been assigned a low confidence score. The remaining ending should be marked as label.
    \item Multiple endings may make sense, but the more plausible ending should be selected. For instance, if a context is "A man is singing into a microphone", then the ending "A man performs a song" will be preferred over the ending "A man is performing on stage" \cite{chen-etal-2020-uncertain}.
\end{enumerate}

For crowdsourcing, we hired graduate student workers who were first given a detailed tutorial on how most plausible ending needs to be identified after which selection was based on a screening test. Examples that were not predicted correctly by a student worker were filtered out, ensuring that each example in \textsc{DiscoSense} has been solved by a human.

\begin{table}[t]
\footnotesize
\centering
% \begin{center}
\begin{tabular}{lccc}
\toprule
Generator & Perplexity \\ 
\midrule
\textsc{GPT2-XL} & 2.53 \\
\textsc{CTRL} & 2.39 \\
\bottomrule
\end{tabular}
\caption{Perplexity scores obtained with generator LMs on the Discovery validation set. Lower is better.}
\vspace{-2mm}
\label{tab:perplexity}
\end{table}

}

\section{Crowdsourcing Details}

We performed crowdsourcing to determine if humans are able to identify the ground truth in each example present in the training and test sets of \textsc{DiscoSense}. 
%For crowdsourcing, we hired undergraduate and graduate student workers who were first given a detailed tutorial on how most plausible ending needs to be identified, after which selection was based on a screening test. 
%Examples that were not predicted correctly by a student worker were filtered out.
%ensuring that each example in \textsc{DiscoSense} has been solved by a human.

\subsection{Selection of Annotators}
We selected undergraduate and graduate student workers primarily on the basis of relevant background knowledge and their current skill set.  %and relevant courses are taken. 
Since the dataset features intricate English sentences, we shortlisted students who are native English speakers. We presented all shortlisted student workers with a one-hour training session followed by an evaluation test and ranked them based on their performance on the test. %picked 
We then hired the top-performing students as our annotators and asked them to answer each example in \textsc{DiscoSense}. 
%for the process of verifying if humans can answer each of the examples in \textsc{DiscoSense} correctly. 
We closely monitored the progress and the performance of each annotator %closely 
and provided timely feedback through virtual meetings on how his/her way of performing annotation can be improved by understanding the difficulties encountered by him/her and  
%answering questions and 
rectifying any problems if they have been doing the annotation in an incorrect manner. All of the annotators were made aware of how the annotated data would be used and its implications. The student workers who did not perform the annotation work in a satisfactory manner were replaced by the next best performing student on the waitlist. All student workers were paid $\$10$/hr \cite{fort2011amazon,cohen2016ethical}.

\subsection{Instructions Provided to Annotators}

Below are the instructions we presented to the annotators during our one-hour tutorial. Each of them received a copy of these instructions plus numerous examples (one of them is shown below) at the end of the tutorial and was given an opportunity to ask clarification questions about the instructions and the annotation process in general after a closer examination of these instructions and examples.

\paragraph{Motivation.}
Academic research is an exploration activity to solve problems that have not been completely solved before. By this nature, each academic research work must sit at the frontier of the field and present novelties that have not been addressed by prior works. Machine Learning (specifically Deep Learning) has seen advancements in numerous domains such as personal assistants, machine translation, etc. What you may have seen is a particular Machine Learning algorithm being deployed in finished end products, but what we do not observe are the research challenges that were overcome behind the scenes to get there. What you will be involved in is one of the research tasks that is far from being solved. You will be contributing towards a meaningful task that has the potential to make scientific advancements.
We are dealing with Commonsense Reasoning with regard to Natural Language Processing. Specifically, we are addressing the problem of how machines can learn to reason in the manner humans do with textual data. This task often requires humans to make use of the information they have acquired about our world (e.g., how the physical world works), and reason about what they read and how it complies with what they already know. The reasoning works on multiple levels: firstly we understand the information we read, make sure we understood it properly, and then reason through various means about it to ensure that it makes sense with what we know. The following quote sums it up nicely. \\ 

\fbox{\begin{minipage}{17em}
The brain is an abduction machine, continuously trying to prove abductively that the observables in its environment constitute a coherent situation. 

\vspace{2mm}
--- Jerry Hobbs, ACL 2013 Lifetime Achievement Award winner
\end{minipage}}
\newline
\\ \\ Current Deep Learning models are very good at picking unintended signals to arrive at the correct answer, but this is not what we intend them to do.
For instance, if ``not" is present within a sentence, then the model might be biased towards predicting negation even though that might not be the case.
We require them to pick the right answer %in the same way which is 
through a reasoning process that is as close to the human reasoning process as possible.
%how humans would do. 
To address this task, we need to build a dataset that aims at providing ``correct" signals to our models, and hopefully the models can learn to reason reasonably well once they are trained on this dataset.

\paragraph{High level description of the task.} 
The task description is straightforward.\\ \\
\fbox{\begin{minipage}{18em}
Given a context and a discourse connective,\\ 
predict which ending is the best to the best\\
of your knowledge/capability.
\end{minipage}}
\newline
\\

While reading the contexts, you %are also supposed to 
should understand what the discourse connective is supposed to convey.
A discourse connective is a word/phrase 
used to connect two sentences and reveal their relationship. 
Consider the following examples.
\begin{enumerate}
    \item \textcolor{teal}{I am feeling hungry}, \textbf{as a result}, \textcolor{orange}{I cooked lunch}.
    \item \textbf{Although} \textcolor{teal}{I liked reading the book}, \textcolor{orange}{there were some major flaws}.
\end{enumerate}
%"as a result" and "although" are the discourse connectives.

In these examples, the green-colored text is the context and the discourse connective is boldfaced. Notice how the text in orange is framed in accordance with the discourse connective. For instance, if ``as a result" is present, then the ending will most likely be about the consequence of what is described in the context; in contrast, if ``although" is the discourse connective, then the ending needs to take a contrasting standpoint. Hence, the discourse connective decides what the ending needs to talk about.
We have provided a list of the discourse connectives you can expect in the ``Role of discourse connectives" section. You are required to be completely familiar with the role each
connective is supposed to play.

Figure~6 shows an example you might expect in the dataset.
%(more examples were presented and discussed during the tutorial):
Any ending that violates what we know about how the physical world works or challenges our notions about anything in particular needs to be discarded.
You have to choose the most plausible ending, which is the ending that is the most feasible amongst four endings. In cases where two or more endings seem equally feasible, the following criteria should be used.

% \twocolumn
\begin{figure}[t!]
\centering
\footnotesize
\begin{subfigure}[b]{0.475\textwidth}
\centering
    {\FrameSep1pt
    \begin{framed}\small\begin{tabular}{@{}l @{}}
\aquestion{}{I love that he’s able to use wired as a venue for launching future
bestsellers \discourse{though}}{a) I think the wired article is a bit too long.}{b) I don’t think its a bad thing for him to do so.}{c) I do agree with some of the other reviews that wired is not a very well written book.}{\correctans{d) Honestly, I might have preferred the podcast of his presentation on the topic.}}
\end{tabular}
\end{framed} }
\end{subfigure}

\comment{
\begin{subfigure}[b]{0.475\textwidth}
{\FrameSep1pt
    \begin{framed}\scriptsize\begin{tabular}{@{}l @{}}
\aquestion{}{\textbf{2.} Dependents are not generally permitted to accept employment. \discourse{Because of this}}{\correctans{a) Students may find that they cannot support a family while
              studying at the university and must be prepared to leave family
              in the home country.}}{b) They cannot be rehired for another position within this company.}{c) The company is unable to recruit new employee at this time.}{d) They are often forced to seek work in the underground economy.}
\end{tabular}
\end{framed} }
\end{subfigure}
}
% \onecolumn
\caption{Example taken from the \textsc{DiscoSense} training set. The correct answer is {\bf boldfaced}.} %) is the one that is most plausible amongst all.}
\label{fig:teaser_examples}
\end{figure}

\begin{itemize}
    \item Any ending that seems to be indisputably correct can be regarded as the best. 
    %For instance, In the above example, In \texttt{Example 3},  option 3 is an example of what a challengeable option looks like. On the contrary, option 1 seems to be better aligned with our understanding and less likely to be disputed. We are more interested in statements that the majority of us can agree on, opinions that are less likely to be challenged.
    \item The best ending will not be inconsistent with the context and the discourse connective. 
%    \item The best ending has to comply with the discourse connective. 
    \item If all three options seem incorrect and implausible and the remaining option makes the most sense relatively, then it should be chosen since the correct ending is the best ending by default.
    \item Two endings can make sense, but the ending that is likely to be more sensible is what you should consider as the best. For example:
    \begin{itemize}
        \item Context: A man is singing into a microphone.
        \item Ending 1: A man performs a song.
        \item Ending 2: A man is performing on stage.
    \end{itemize}
Ending 2 is not incorrect but ending 1 makes more logical sense to us as humans. In such cases, mark what seems more logical to you.
\end{itemize}

\paragraph{Role of discourse connectives.}
Please make sure that you understand the role of each connective.
\begin{itemize}
\item although: in spite of the fact that; even though
\item as a result: because of something
\item because of this: for the reason that
\item because of that: for the reason that
\item but: used for joining two ideas or statements when the second one is different from the first one
\item by contrast: used to express difference with something
\item consequently: as a result
\item conversely: introducing a statement or idea which reverses one that has just been made or referred to
\item for example: used to introduce something
\item for instance: as an example
\item hence: as a consequence; for this reason
\item however: used to introduce a statement that contrasts with or seems to contradict something that has been said previously
\item in contrast: used to express difference with something
\item in other words: to put it another way
\item in particular: especially; specifically
\item in short: to sum up; briefly
\item in sum: to sum up; in summary
\item instead: as an alternative or substitute
\item interestingly: in a way that arouses curiosity or interest
\item likewise: in the same way
\item nevertheless: in spite of that; notwithstanding; all the same 
\item nonetheless: in spite of that; nevertheless
\item on the contrary: conversely; used to intensify a denial of what has just been implied or stated by suggesting that the opposite is the case
\item on the other hand: used to introduce a contrasting point of view, fact, or situation
\item otherwise: in circumstances different from those present or considered; or else
\item overall: taking everything into account
\item particularly: especially
\item rather: used to indicate one's preference in a particular matter; preferably
\item similarly: in a similar way
\item specifically: in a way that is exact and clear; precisely
\item subsequently: after a particular thing has happened; afterward 
\item thereafter: after that time
\item thereby: by that means; as a result of that
\item therefore: for that reason; consequently
\item though: despite the fact that; although
\item thus: as a result or consequence of this; therefore
\item yet: so far; up until the present or a specified or implied time; by now or then
\end{itemize}

\comment{
\section{State-of-the-Art Results on Other Commonsense Reasoning Benchmarks}

One of the motivations behind the creation of \textsc{DiscoSense} was that state-of-the-art PLMs have managed to achieve or even surpass human performance on the vast majority of well-known commonsense reasoning benchmarks. To make this statement more concrete, we show in Table~\ref{tab:status_difficulty_benchmark} the best accuracy achieved by existing PLMs and the corresponding human performance on eight of the widely used commonsense reasoning benchmarks.

\begin{table}[h!]
\begin{small}
\centering
\setlength{\tabcolsep}{2.5pt}
\begin{tabular}{lcccc}
  \toprule
  Dataset & Model & Human \\
  \midrule
%   \multicolumn{5}{l}{\emph{Small models}}\\
  SWAG \cite{zellers-etal-2018-swag} & 91.71 & 88\\
  $\alpha$NLI \cite{bhagavatula2020abductive} & 91.18 & 92.9\\
  Hellaswag \cite{zellers-etal-2019-hellaswag} & 93.85 & 95.6 \\
  CosmosQA \cite{huang-etal-2019-cosmos} & 91.79 & 94\\
  PIQA \cite{Bisk2020} & 90.13 & 94.9\\
  SocialIQA \cite{Sap2019SocialIC} & 83.15 & 88.1\\
   MC-TACO  \cite{zhou-etal-2019-going} & 80.87 & 75.8\\
  WinoGrande \cite{Sakaguchi2020WINOGRANDEAA} & 86.64 & 94 \\
%  ProtoQA & 54.15 & 74.03\\
%  VCR & 63.15 & 85\\
  \bottomrule
\end{tabular}
  \caption{
    Status of how competitive current commonsense reasoning benchmarks are for SoTA models. Most of them are close to being entirely solved.
  }
\label{tab:status_difficulty_benchmark}
\end{small}
\end{table}

\section{Hyperparameter Tuning }

We perform hyperparameter tuning of the baseline models to determine parameters which work well. 
The search range is in part guided by 
%Most of the parameters that worked well do not diverge much from 
the default ones provided in \cite{DBLP:journals/corr/abs-1910-03771}. 
We ran our hyperparameter search trial five times on the dev set, this means that the model would be trained five times and its performance would be observed on the dev set to determine which parameters worked the best. Hyperparameters were determined based on the accuracy obtained by the model on the dev split of \textsc{Discosense}.
\begin{itemize}
    \item A higher batch size (i.e 16) helps with the optimization of the model. Smaller batch sizes can cause instability in the early course of training.
    \item We find that having a large warmup steps helps the model in stabilization and obtain improved performance on this dataset. 
    \item We sample learning rates between $1e-5$ to $5e-5$ using log-uniform distribution to determine how warmup takes place and how well the model is able to adapt to this training regime. We find that a learning rate of $2e-5$ worked the best for both models.
    \item We find that a having a higher number of epochs (i.e 8) helps the Conditional Adversarial Filtering process. Even after 4 epochs, the discriminator LM observes performance improvements which allows it to filter out more easy examples.
\end{itemize}

\begin{table} [t]
\begin{center}
\footnotesize{
\begin{tabular}{|l|r|}
\hline
\multicolumn{1}{|c|}{Hyperparameter} & \multicolumn{1}{c|}{Value}  \\
\hline
Learning rate &  $2e-5$\\
gradient accumulation & 1\\
weight decay & 0 \\
adam beta 1 & 0.9 \\
adam beta 2 & 0.99 \\
num train epochs & 8 \\
lr scheduler & linear \\
warmup steps & 8000 \\
\hline

\end{tabular}}
\end{center}
\caption{Hyperparameter configurations of the best performing models.}
\label{tab:hyperparameter-config}
\end{table}
}

% \section{Examples}
% In this section, we demonstrate examples from \textsc{Discosense} targeting different categories of commonsense reasoning.

% \begin{figure}[t]
% \centering\footnotesize

% \caption{Social Example}
% \caption{Example questions answered by BERT-Large. Correct model predictions are \correctans{blue}, incorrect predictions are \incans{red}. The right answers are \textbf{bolded}.}
% \label{tab:social_example_main}
% \end{figure}

% \section{Examples}
% \label{sec:all_data_examples}
% In this section, we provide examples from training set of \textsc{Discosense} belonging to numerous categories such as physical world (~\autoref{tab:physical_world_examples}), social (~\autoref{tab:social_examples}), linguistic (~\autoref{tab:linguistic_examples}), numerical (~\autoref{tab:numerical_examples}), temporal (~\autoref{tab:temporal_examples}) and abductive (~\autoref{tab:abductive_examples} reasoning.
%\vspace{2cm}

\comment{
\begin{figure}[h]
\centering\footnotesize
    {\FrameSep1pt
    \begin{framed}\scriptsize\begin{tabular}{@{}l @{}}
\aquestion{}{The 365 feet tall megasaur isnt our enemy, out to destroy humanity like in the original movie  \discourse{instead}}{a) He is our friend}{b) His intent on restoring natures balance in a world that has been neglected and abused by humans. }{c) His is our best hope to return the world to its original glory.}{\correctans{d) This movie is about the aliens need to conquer earth in an eventual destruction at the hands of man and his technology.}}
\end{tabular}
\end{framed} }
{\FrameSep1pt
    \begin{framed}\scriptsize\begin{tabular}{@{}l @{}}
\aquestion{}{It would certainly be interesting to take off with an umbrella and fly over the feed yard in the wind,  \discourse{although}}{a) Since the wind is so nice, I guess that would be pretty dangerous}{b) The temperature was very warm and the breeze was quite refreshing.}{\correctans{c) I would have to look fast because it wouldnt take long for me to be at the kansas border with the terrible winds that we have experienced lately.}}{d) I am not sure id want to get caught in one of those things.}
\end{tabular}
\end{framed} }
{\FrameSep1pt
    \begin{framed}\scriptsize\begin{tabular}{@{}l @{}}
\aquestion{}{I could not tell whether the smell was coming from my room or wafting in through the vents. \discourse{On the other hand}}{a) The sheets, towels, and bathroom seemed clean, which is, of course, whats important}{b) I can smell the stinky air freshener that my mother keeps in her room.}{\correctans{c) I had another visitor who was not so lucky.}}{d) I had a similar experience when I was about ten years old. I used to have to sleep with a fan running to drown out the stifling smell.}
\end{tabular}
\end{framed} }
{\FrameSep1pt
    \begin{framed}\scriptsize\begin{tabular}{@{}l @{}}
\aquestion{}{The molecules in a moisturizer are larger than the molecules in a serum. \discourse{Because of this}}{a) A moisturizer will not sink into fine wrinkles and fine lines}{b) The amount of moisturizer is more than enough to make a difference}{\correctans{c) The moisturizer cannot penetrate the skin as deep as a serum can}}{d) Larger molecules, the serum cannot penetrate deeply into the moisture.}
\end{tabular}
\end{framed} }
\vspace*{-3mm}
\caption{Physical World Reasoning Examples from \textsc{Discosense} training set.}
\label{tab:physical_world_examples}
\end{figure}

\begin{figure}[t]
\centering\footnotesize

  {\FrameSep1pt
    \begin{framed}\scriptsize\begin{tabular}{@{}l @{}}
\aquestion{}{If there is a problem putting your carts in the street, please put your carts as close as possible to the street. \discourse{For example}}{\correctans{a) In your driveway, on the mow strip, or at the edge of the sidewalk.}}{b) In the event of an accident involving a pedastrian or cyclist, please move your cart as far as possible.}{c) If you have a hard time putting the carts on the sidewalk}{d) If you live in an apartment building and have a small car, please put both your carts as near the curb as possible.}
\end{tabular}
\end{framed} }
\vspace*{-3mm}

{\FrameSep1pt
    \begin{framed}\scriptsize\begin{tabular}{@{}l @{}}
\aquestion{}{A small circle of specialists makes trade policy, often with a disproportionate amount of influence from those with a direct economic benefit. \discourse{In sum}}{\correctans{a)  Policymakers have developed an efficient trade development process but that process has not created public support and understanding }}{b) I would say that the current situation is not sustainable.}{c) It is in the interests of the united states to have an informed and engaged citizenry that is well informed about trade and the policy issues that affect its interests.}{d) While trade is an important aspect of economic policy, it is not the only aspect.. }
\end{tabular}
\end{framed} }

    {\FrameSep1pt
    \begin{framed}\small\begin{tabular}{@{}l @{}}
\aquestion{}{I love that he's able to use wired as a venue for launching future bestsellers \discourse{though}}{a) I think wireless might be the way to go for him in that he can continue to attract fans and sell more of his own books. }{b) I am not a fan of his last two books, so i don't think he will be writing any more of me.}{c) His last two albums were great, his latest album is a bit more disappointing compared to the first three.}{\correctans{d) Honestly, I might have preferred the podcast of his presentation on the topic.}}
\end{tabular}
\end{framed}}
    {\FrameSep1pt
    \begin{framed}\small\begin{tabular}{@{}l @{}}
\aquestion{}{For the last 4 years he has suffered from very bad depression \discourse{although}}{a) He is now very much better, he still has bad days the day before he had severe depression, he was very happy}{b) He is still very active and healthy physically and mentally.}{\correctans{c) I only discovered that this is what it actually was maybe a year ago}}{d) He is not in danger of losing his house, he is still very poor.}
\end{tabular}
\end{framed} }

 {\FrameSep1pt
    \begin{framed}\small\begin{tabular}{@{}l @{}}
\aquestion{}{The department of residence life at university of wisconsin platteville values the impact that parents and families have on our students. \discourse{Because of this}}{a) Our faculty and staff are committed to providing clinical instruction that helps our students develop the knowledge and understanding of the clinical care and management they will need as adults.}{b) We believe that student success is directly related to the academic environment that surrounds our schools.
}{c) We believe in creating a welcome, supportive and challenging environment for all students.)}{\correctans{d) We provide access to the campus link, a monthly publication targeted to the parents and families of our residence hall students.}}
\end{tabular}
\end{framed} }

 {\FrameSep1pt
    \begin{framed}\small\begin{tabular}{@{}l @{}}
\aquestion{}{In fact, just today a friend of mine committed a certain amount for two months for the radio show. \discourse{Therefore}}{a) I am on the road to recovery.}{b) He did not get paid at all.
}{\correctans{c) We have enough for me to do a five day a week, 1-2 hour a day, for about two months.)}}{d) My blog is mostly written about what is going on with the show.}
\end{tabular}
\end{framed} }

\vspace*{-3mm}
\caption{Social Reasoning Examples from \textsc{DiscoSense} training set.}
\label{tab:social_examples}
\end{figure}

\begin{figure}[t]
\centering\footnotesize

{\FrameSep1pt
    \begin{framed}\scriptsize\begin{tabular}{@{}l @{}}
\aquestion{}{The data reported by each respondent are not readily comparable among countries. \discourse{For example}}{a)  In australia, the abs collects data on both telephone and web site use, but that are available for all countries}{b) Although in some european countries the use of antiretroviral therapy may be more common than in the United States.}{c) Some of the respondents may not have reported any data at all for any of their countries.}{\correctans{d) Some respondents reported data for the year 2005, while others reported data for the year 2006.}}
\end{tabular}
\end{framed} }

    {\FrameSep1pt
    \begin{framed}\scriptsize\begin{tabular}{@{}l @{}}
\aquestion{}{Because expression of this gene is much more robust in male species, 323.3, we excluded possibility of sample mixup; \discourse{therefore}}{a) We were not able to detect the presence of 317.}{\correctans{b) We considered that values equal or below the 8.1 threshold were not reliable.}}{c) We have re analyzed our data using male and female species seperately.}{d) We generated 3 new samples from 3 males each.}
\end{tabular}
\end{framed} }

{\FrameSep1pt
    \begin{framed}\scriptsize\begin{tabular}{@{}l @{}}
\aquestion{}{While small in number, the population had been there for several years. \discourse{Interestingly}}{a) The population grew in the same area where they had lived all those years.}{b) There is no evidence of any recent human activity and very little has been done in the way of infrastructure.}{\correctans{c) The population contained both european and the native eastern oysters.}}{d) During the war, the indians made a pact with the government of Oklahoma city and agreed to leave the area if the war ended .}
\end{tabular}
\end{framed} }

{\FrameSep1pt
    \begin{framed}\scriptsize\begin{tabular}{@{}l @{}}
\aquestion{}{Facebook boasts more than 500 million active users, while linkedin has more than 100 million members \discourse{as a result}}{a) Linkedin is the runner up of the annual best online b2b awards presented by the association of technology officers in this year.}{b) The companies have become key to the obama administrations new marketing offensive.}{\correctans{c) Savvy staffing firms are creating company facebook pages or tweeting to attract top notch candidates.}}{d) Both are experiencing explosive growth, with linkedins numbers approaching those of Facebook.}
\end{tabular}
\end{framed} }

% {\FrameSep1pt
%     \begin{framed}\scriptsize\begin{tabular}{@{}l @{}}
% \aquestion{}{The number of students who graduated with degrees in nursing increased by about 13.8\% from 2008 to 2010 \discourse{in particular}}{a) The number of undergraduate students did not go up.}{\correctans{b) The number of undergraduate students climbed up by 77 students.}}{c) The total number of undergraduate students went up by two students.}{d) The percent of undergraduate students increased from 46\% to 54\%.}
% \end{tabular}
% \end{framed} }

\vspace*{-3mm}
\caption{Numerical Reasoning Examples from \textsc{Discosense} training set.}
\label{tab:numerical_examples}
\end{figure}

\begin{figure}[t]
\centering\footnotesize
    {\FrameSep1pt
    \begin{framed}\scriptsize\begin{tabular}{@{}l @{}}
\aquestion{}{Participants were instructed not to change their training intensity or volume, thus no overload throughout the duration of the study occurred \discourse{as a result}}{a) The subjects were encouraged to maintain a consistent training volume throughout their study, a key component to the long term effectiveness of this intervention.}{b) There was no significant change in training load or time in the three week period following treatment}{\correctans{c) No effect of the training or hmb ca was observed on indices of damage.)}}{d) Participants decreased their bmd only slightly over the 8 week period. }
\end{tabular}
\end{framed} }
   {\FrameSep1pt
    \begin{framed}\scriptsize\begin{tabular}{@{}l @{}}
\aquestion{}{Similary, our findings, as well as those of kern et al. did not link ae with hunting \discourse{in contrast}}{a) In our data we haev found evidence that hinting ability is positively related to the expression of a homeodomain transcription factor in an h3k9 gene.}{\correctans{b) A previous study in Austria identified hinting as the most notable observed risk factor}}{c) In our study we found that most ae did contribute to hunting in a significant way.)}{d) However, our data show that the ne of the environment is a significant predictor of hunting success.}
\end{tabular}
\end{framed} }

 {\FrameSep1pt
    \begin{framed}\scriptsize\begin{tabular}{@{}l @{}}
\aquestion{}{We work diligently to maintain a pest free facility \discourse{therefore}}{\correctans{a) We request that all canine guests be treated with a quality flea and tick preventative prior to visiting our salon}}{b) All pest control materials are disinfected prior to being placed in the storage facility.}{c) We are not responsible for the pest control issues the may occur on our propery.)}{d) All pest control services are free of charge.}
\end{tabular}
\end{framed} }

{\FrameSep1pt
    \begin{framed}\scriptsize\begin{tabular}{@{}l @{}}
\aquestion{}{The book is filled with carefully crafted poems like this one, in which tradition and innovation, chaos and order, and even michael bolton coexist gracefully within the same rhetorical space. \discourse{In short}}{a) They have a very nice view on the world.}{b) The poetry in this collection is a tour de force of literary invention and subtle social commentary.}{\correctans{c) A wonderful collection from a gifted poet.}}{d) Boltons ability to make seemingly disparate materials cohere into a single work of art is something to be marveled at..}
\end{tabular}
\end{framed} }

\vspace*{-3mm}
\caption{Linguistic Reasoning Examples from \textsc{Discosense} training set.}
\label{tab:linguistic_examples}
\end{figure}

\begin{figure}[t]
\centering\footnotesize
   
   {\FrameSep1pt
    \begin{framed}\scriptsize\begin{tabular}{@{}l @{}}
\aquestion{}{After that, I moved down to Florida, 3 years ago, and, unfortunately, rushed into a marriage after only 6 months. \discourse{Because of that}}{a) I have always been vary of commitment.}{\correctans{b) I want to take a new relationship very slowly.}}{c) I have a 2 year old and I was pretty irresponsible and didn't think through the consequences of getting married.}{d) We were not able to have any children, and I had to get an abortion, which I am still paying for today, after 33 years.}
\end{tabular}
\end{framed} }

{\FrameSep1pt
    \begin{framed}\scriptsize\begin{tabular}{@{}l @{}}
\aquestion{}{Not long ago, many people worked on farms or in factories, so they had similar lifestyles \discourse{but}}{\correctans{a) Now the economy rewards specialization, so workplaces and lifestyle changes.}}{b) They were often much poorer.}{c) Now we have a whole new group of people coming to our area and our jobs are being of great importance to them.}{d) Now that the recession has hit, many of these workers are finding themselves in a tough spot.}
\end{tabular}
\end{framed} }

{\FrameSep1pt
    \begin{framed}\scriptsize\begin{tabular}{@{}l @{}}
\aquestion{}{Women over the age of 30 are generally considered to be past the acceptable age for marriage. \discourse{Consequently}}{a) They are not eligible to marry under the law.}{b) Women in this category are likely to have entered into pre-marital agreements well before the legal age at which marriage is compulsory.}{\correctans{c) Although the increase in late marriages affects both sexes, women tend to suffer more from the phenomenon.}}{d) A minimum of 25 years is generally accepted as the minimum age to mary, but this is not always the case.}
\end{tabular}
\end{framed} }

{\FrameSep1pt
    \begin{framed}\scriptsize\begin{tabular}{@{}l @{}}
\aquestion{}{Announced the county courthourse will be closed saturday and monday for the labor day weekend. \discourse{Because of that}}{\correctans{a) The deadline to receive a discount for early property tax payments has been extended from sept. 2 to sept. 3.}}{b) The office will not be open for business on Wednesdays.}{c) The washtenaw country clerks office will operate with one staff member.}{d) The hearing will not be held until next Tuesday July 19..}
\end{tabular}
\end{framed} }

\vspace*{-3mm}
\caption{Temporal Reasoning Examples from \textsc{Discosense} training set.}
\label{tab:temporal_examples}
\end{figure}

\begin{figure}[t]
\centering\footnotesize
    {\FrameSep1pt
    \begin{framed}\scriptsize\begin{tabular}{@{}l @{}}
\aquestion{}{If you have a really fast car, you can just get in the old car, then quickly get out and get back in your fast car and speed to schottler \discourse{nonetheless}}{a) Its still a fun event}{b) You may have to park your old car and walk around a bit. }{c) Schotler is worth the drive because its right next door to the schroeder center and you get a great deal on schrotter beer for 10 bucks a growler.}{\correctans{d) Once youre there, get out of the car and go in to the alleyway under the expressway to find your contract.}}
\end{tabular}
\end{framed} }

{\FrameSep1pt
    \begin{framed}\scriptsize\begin{tabular}{@{}l @{}}
\aquestion{}{Suffers at long range \discourse{though}}{a) A lot of this is dependent on your actual win rate and how well you know your opponent.}{\correctans{b) Due to scatter of shells}}{c) Not really a good option for a beginner.}{d) He does have a powerful attack that can be used to summon the beast of the sea.}
\end{tabular}
\end{framed} }

{\FrameSep1pt
    \begin{framed}\scriptsize\begin{tabular}{@{}l @{}}
\aquestion{}{His being sidelined is definitely unfair \discourse{nonetheless}}{a) I dont think his absence is a huge blow to the team.}{b) It is what it is.}{\correctans{c) He is a true warrior and will never quit.}}{d) He should have been given a red card for that foul which was clearly deliberate.}
\end{tabular}
\end{framed} }

{\FrameSep1pt
    \begin{framed}\scriptsize\begin{tabular}{@{}l @{}}
\aquestion{}{Dont even get me started on that one \discourse{although}}{\correctans{a) Considering the kind of stuff that gets our readers going okay, you got it.}}{b) You are all so you can all eat cake.}{c) I do have a few friends who have the same tissue.}{d) I do like the idea of making a game out of this and making it different every time you play it, but how could they possibly be fun.}
\end{tabular}
\end{framed} }

\vspace*{-3mm}
\caption{Abductive Reasoning Examples from \textsc{Discosense} training set.}
\label{tab:abductive_examples}
\end{figure}
}

\comment{\begin{subfigure}[b]{0.475\textwidth}
{\FrameSep1pt
    \begin{framed}\scriptsize\begin{tabular}{@{}l @{}}
\aquestion{}{\textbf{2.} Now all this has led to a speculation as to just where Deepmind
            might fit among Google's range of services. \discourse{For instance}}{a) Deepmind is said to be working on a virtual assistant that will
               help people complete everyday tasks.}{b) Deepmind  might  be  used  to  power  Google’s  new virtual
              assistant service which is currently in limited beta.}{c) Google  just  bought  boston  dynamics,  its  a  company that
             makes the big dog robot.}{d) It seems that deepmind is developing a virtual assistant that would
             learn and behave like a real person.}
\end{tabular}
\end{framed} }
\end{subfigure}
}
